# Supplementary material for: Free-energy landscapes in magnetic systems from metadynamics
Source: arXiv:1706.10216 source file (2017-10-30)
Supplement: Supplementary file 1 [file supplemental.pdf]

# Free-energy landscapes in magnetic systems from metadynamics - supplemental material.

Jaroslav Tóbik[1], Roman Martoňák[2], and Vladimír Cambel[1]

[1] *Institute of Electrical Engineering, Slovak Academy of Sciences, Dúbravská cesta 9, SK-841 04 Bratislava, Slovakia*

[2] *Department of Experimental Physics, Faculty of Mathematics, Physics and Informatics, Comenius University in Bratislava, Mlynská dolina F2, 84248 Bratislava, Slovakia*

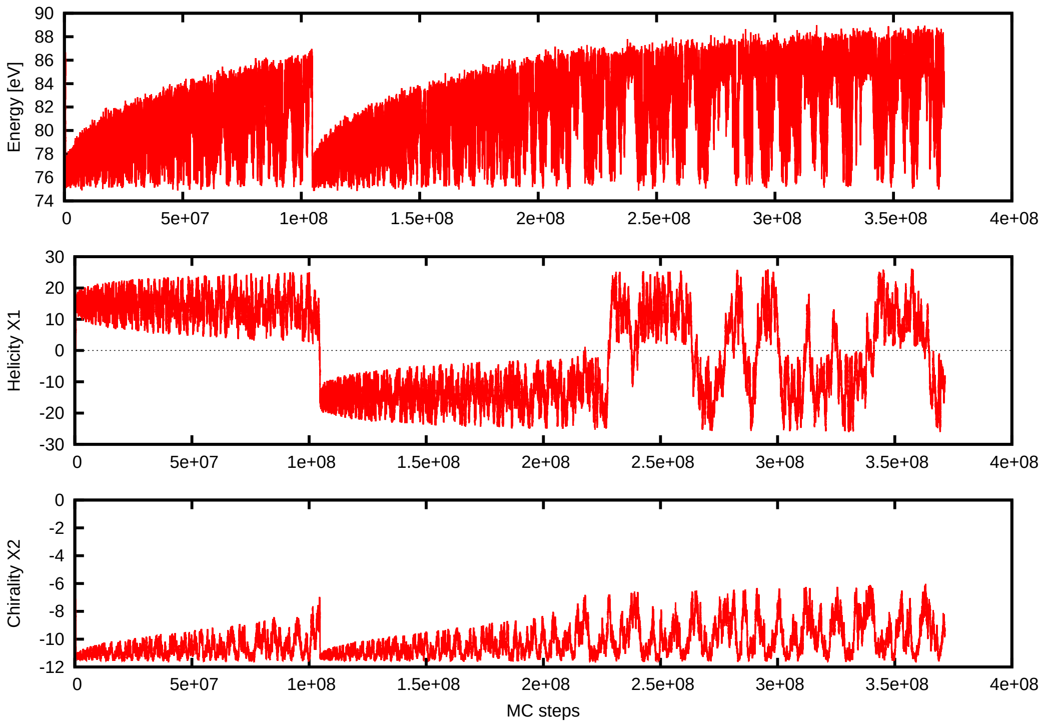


FIG. 1. Time evolution of energy (Eq. 1), helicity $X_1$ (Eq. 4a) and chirality $X_2$ (Eq. 4b) as function of the number of MC steps in metadynamics for initial C state. The reconstructed free energy landscape from this run is shown in the Fig. 1 in the paper.

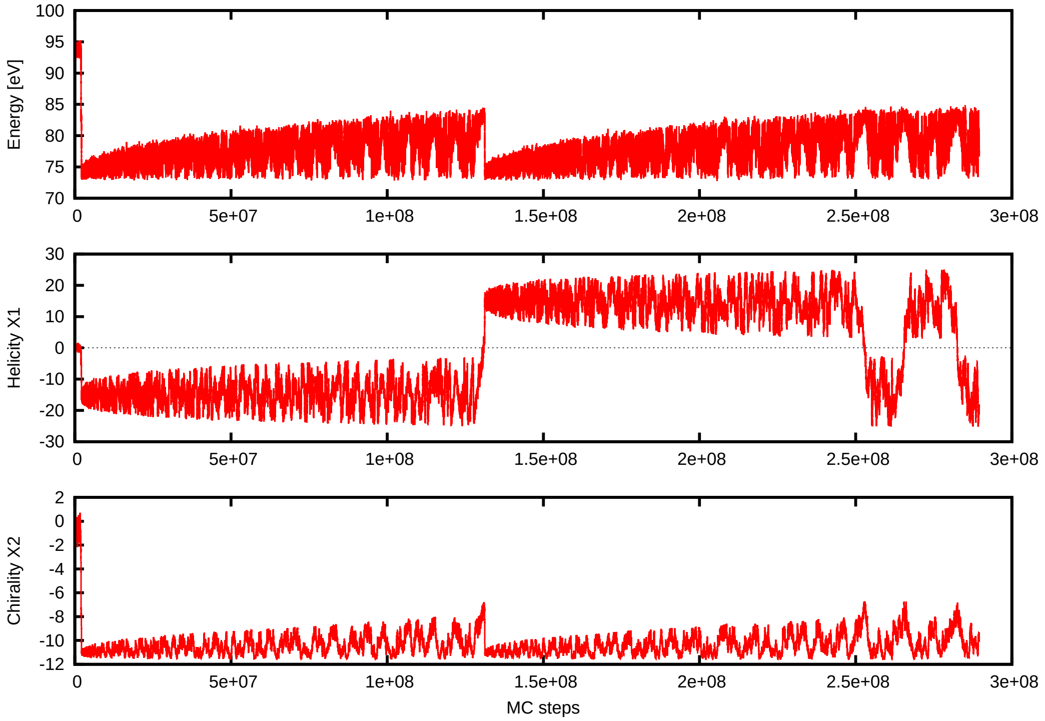


FIG. 2. Time evolution of energy (Eq. 1), helicity $X_1$ (Eq. 4a) and chirality $X_2$ (Eq. 4b) as function of the number of MC steps in metadynamics for initial S state. The reconstructed free energy landscape from this run is shown in the left panel of the Fig. 2 in the paper.

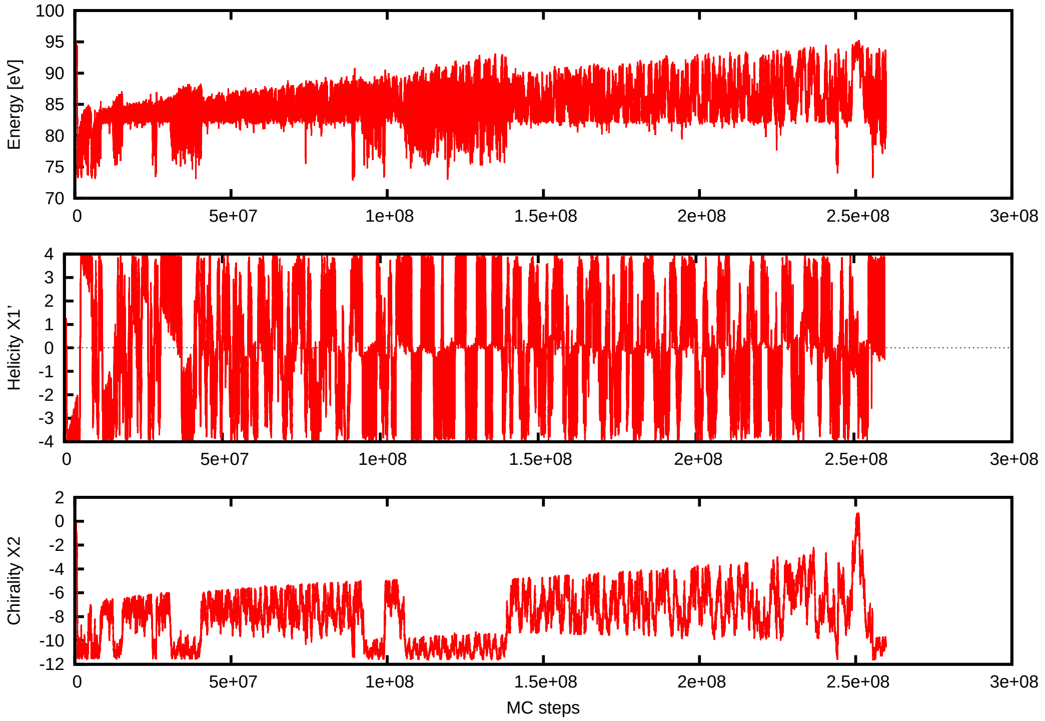


FIG. 3. Time evolution of energy (Eq. 1), transformed helicity $X_1'$ (Eq. 4a') and chirality $X_2$ (Eq. 4b) as function of the number of MC steps in metadynamics for initial S state. The reconstructed free energy landscape from this run is shown in the right panel of the Fig. 2 in the paper.

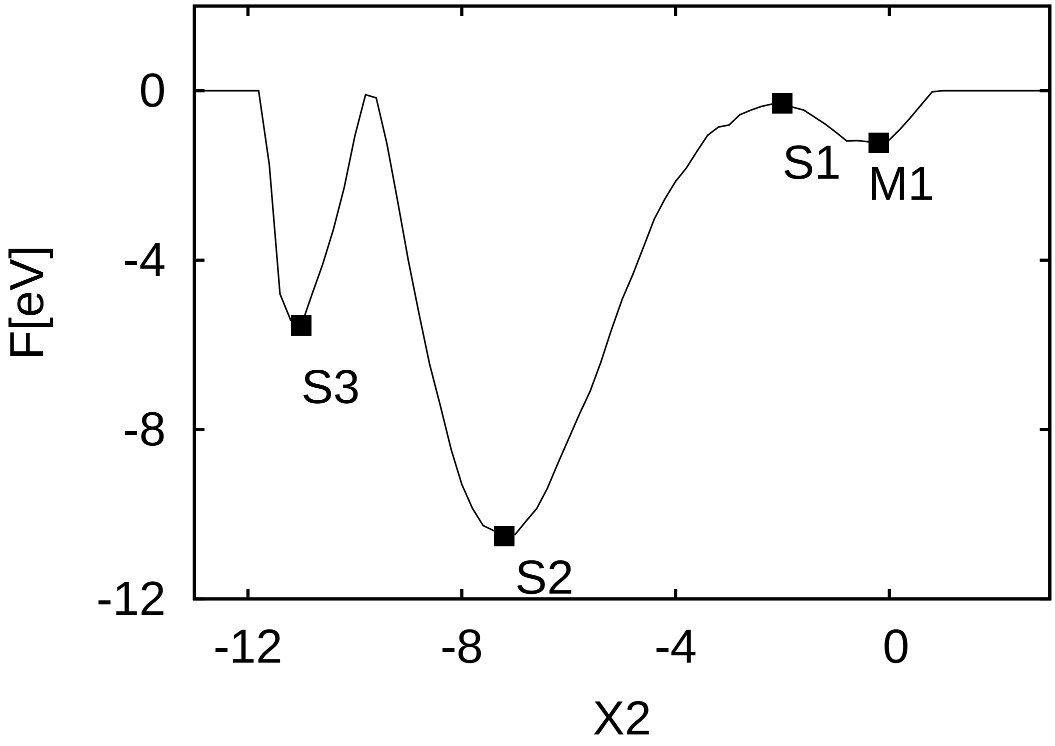


FIG. 4. Profile of the free energy map along symmetry line $X_1' = 0$. The labels of the special points corresponds to the notation in the Fig. 2 in the paper.
